# Supplementary material for: Asymptotically Optimal Welfare of Posted Pricing for Multiple Items with MHR Distributions
Source: arXiv:2107.00526 source file (2021-07-01)
Supplement: Supplementary file 3 [file appendix_additive_static.tex]

% !TEX root = mhr-prophet.tex
\section{Static Pricing for Additive Valuations}
\label{appendix:additive_static}

The notation for additive valuation functions can be found in Appendix \ref{appendix:additive_dynamic}. For the case of static prices, we give a $1 - O \left( \frac{\log\log\log n}{\log n}\right)$-competitive mechanism which is also asymptotically tight by Section \ref{section:optimality}. To this end, for any item, we set the price of item $j$ to \[ p_j = F_j^{-1} \left( 1 -  \frac{\log \log n}{n} \right) \enspace, \] where $F_j^{-1}$ denotes the quantile function of the distribution $\mathcal{D}_j$. This corresponds exactly to the pricing structure in Section \ref{section:independent_valuations_static} and allows us to prove the following theorem.

\begin{restatable}{theorem}{staticadditive}
	\label{theorem:static_additive}
	The posted-prices mechanism with additive buyers and static prices is $1 - O \left( \frac{\log\log\log n}{\log n} \right)$-competitive with respect to social welfare. 
\end{restatable}

\begin{proof}
	We begin with an application of Lemma~\ref{lemma:quantiles1} to get a bound on $p_j$.
	\begin{align*}
	p_j & = F_j^{-1} \left(1- \frac{\log \log n}{n}  \right) \geq \frac{- \log \log \log n + \log n}{H_n} \Ex[]{\max_{i \in [n]} v_{i,j}}  \\ & \geq \left( 1 - \frac{\log \log \log n + 1}{\log n} \right) \Ex[]{\max_{i \in [n]} v_{i,j}} .
	\end{align*} 
	Further, we aim to bound the probability of selling item $j$ in our mechanism. To this end, observe that by additivity, any buyer $i$ buys item $j$ as soon as $v_{i,j} > p_j$ and does not buy item $j$ otherwise independent of all other items $j'$. As a consequence, we can bound the probability of not selling item $j$ via \[ \Pr[]{j \text{ unsold}} = \prod_{i=1}^{n}  \left(1- \frac{\log \log n}{n} \right) =  \left(1- \frac{\log \log n}{n}  \right)^n \leq \frac{1}{\log n} \enspace. \]
	
	Therefore, the probability of selling item $j$ in our mechanism is at least $\Pr[]{j \text{ sold}} \geq 1 - \frac{1}{\log n}$. This allows to bound the expected revenue of our mechanism by a suitable fraction of the optimal social welfare.
	
	\begin{align*}
	\Ex[]{\ALG} & \geq \Ex[]{\revpp} = \sum_{j=1}^{m} \Pr[]{j \text{ sold}} \cdot p_j \\ & \geq \sum_{j=1}^{m} \left( 1 - \frac{1}{\log n} \right) \left( 1 - \frac{\log \log \log n + 1}{\log n} \right) \Ex[]{\max_{i \in [n]} v_{i,j}} \\ & \geq \left( 1 - O \left( \frac{\log\log\log n}{\log n} \right) \right) \Ex[]{\OPT} \ .
	\end{align*}	
	
\end{proof}

Observe that the proof of Theorem \ref{theorem:static_additive} only requires to bound the expected revenue of our mechanism and hence, allows to state the following corollary.

\begin{corollary}
	The expected revenue achieved by the posted-prices mechanism with additive buyers and static prices yields a $1 - O \left( \frac{\log\log\log n}{\log n}\right)$-fraction of the expected optimal revenue. 
\end{corollary}
