# Supplementary material for: Asymptotically Optimal Welfare of Posted Pricing for Multiple Items with MHR Distributions
Source: arXiv:2107.00526 source file (2021-07-01)
Supplement: Supplementary file 4 [file appendix_independent_values_dynamic.tex]

\section{Simplified Proof for Section \ref{section:independent_valuations_dynamic} on Independent Valuations for $m \leq n$}
\label{appendix:independent_valuations_dynamic}

We give a simplified proof of Theorem \ref{theorem_independent_dynamic} for the case that $m \leq n$. The full proof for any $m$ can be found in Appendix~\ref{appendix:independent_valuations_dynamic_general}.

\theoremindependentdynamic*

\begin{proof}[Proof of Theorem \ref{theorem_independent_dynamic}, simplified version for $m \leq n$]
	In the following, we assume that $m=n$. If we have less items than buyers, we can add dummy items with value $0$ to ensure $m=n$. Matching $i$ to one of these dummy items in the mechanism then corresponds to leave $i$ unmatched. Observe that from a technical point of view, a point mass on $0$ is not a MHR distribution and hence, the lemmas for MHR distributions do not apply. We will give suitable remarks in the proof when necessary to show how to overcome these problems. 
	
	First, we lower-bound the expected social welfare $\Ex{\ALG}$ of our posted-prices algorithm by the expected social welfare $\Ex[]{\textnormal{SW}_{\textnormal{quantile}}}$ of the following \emph{quantile allocation rule} stated in Algorithm \ref{algorithm_dynamic_independent_2}:\\
	Consider buyer $i$ in step $i$. Instead of allocating buyer $i$ the item that maximizes her utility $v_{i, j} - p_j^{(i)}$ for $j \in M^{(i)}$, we allocate the item that attains the highest quantile $\max_{j \in M^{(i)}} F_j(v_{i, j})$. For any $j$ (which is not a dummy item), $F_j(v_{i, j}) \sim \textnormal{Unif}[0,1]$. \\
	
	\begin{algorithm}[h]
		\SetAlgoNoLine
		\DontPrintSemicolon
		$M^{(1)} \longleftarrow M$ \\
		\For{$i \in N$}{
			\text{Compute $d_{i,j} := F_j(v_{i, j})$ for any $j \in M^{(i)}$ which is not a dummy item} \\ 
			\text{Sample $d_{i,j} \sim \textnormal{Unif}[0,1]$ for dummy items (if present)} \\
			\text{Set $j_i$ such that it attains $\max_{j \in M^{(i)}} d_{i,j}$ and remove $j_i$ from $M^{(i+1)}$ } 
		}
		\caption{Quantile Allocation Rule for Independent Item Valuations}
		\label{algorithm_dynamic_independent_2}
	\end{algorithm}
	
	In the case of having dummy items present, note that $v_{i,j} = 0$ for these dummy items. As a consequence, for any dummy item $j$, we draw an artificial quantile variable $d_{i,j} \sim \textnormal{Unif}[0,1]$ independently and use this sample instead of $F_j(v_{i, j})$ in the Quantile Allocation Rule. By this, we ensure that each item is still allocated with probability $\frac{1}{n-i+1}$ and further one item (maybe a dummy item) is sold for sure. Consequently, the set of remaining items $M^{(i)}$ is identically distributed under the posted-prices mechanism and the quantile allocation rule.
		
	We also claim that the expected contribution of any buyer to the social welfare in the posted-prices mechanism is at least as large as under the quantile allocation rule. To this end, split buyer $i$'s contribution to the social welfare in revenue and utility. The probability of selling a specific item is equal for the two allocation rules, so the expected revenue of both is the same. Further, since we maximize utility in the posted-prices mechanism, the achieved utility is always at least the utility of the quantile allocation rule. So, overall, we get $\Ex[]{\textnormal{SW}_{\textnormal{quantile}}} \leq \Ex{\ALG}$. 
	
	In order to compare the welfare of the quantile allocation rule to the optimal allocation, we introduce indicator variables $X_{i, j}$ which are equal to $1$ if buyer $i$ gets item $j$ in the quantile allocation and $0$ otherwise. 
	
	\[
	\Ex{v_{i, j} X_{i, j}} = \frac{n-i+1}{n} \cdot \frac{1}{n-i+1} \cdot \Ex{v_{i, j} \growingmid X_{i, j} = 1 } = \frac{1}{n} \Ex{v_{i, j} \growingmid X_{i, j} = 1 } \enspace.
	\]
	Now, consider a fixed item $j$ which was chosen according to $\arg\max_{j \in M^{(i)}} F_j\left( v_{i, j} \right)$. Since all items are independent and quantiles follow a $\textnormal{Unif}[0,1]$-distribution, the expected value of item $j$ is the same as if the valuation was the maximum of $n-i+1$ i.i.d. draws from distribution $\mathcal{D}_j$. (Note that in the presence of dummy items, we sampled artificial quantiles $d_{i,j}$ for these in order to ensure this property.) An application of Lemma \ref{Lemma:Babaioff_bound_maximum} leads to\footnote{Again, for dummy items, $\Ex[]{\max_{i' \in \left[n-i+1\right]} v_{i', j} } = \Ex[]{\max_{i' \in [n]} v_{i', j}}= 0$ and hence, the same bound holds.}
	\begin{align*}
	\Ex{v_{i, j} X_{i, j}} = \frac{1}{n} \Ex{v_{i, j} \growingmid X_{i, j} = 1 } = \frac{1}{n} \ \Ex[]{\max_{i' \in \left[n-i+1\right]} v_{i', j} } \geq \frac{1}{n} \cdot \frac{H_{n-i+1}}{H_n} \cdot \Ex[]{\max_{i' \in [n]} v_{i', j}}
	\end{align*}
	Note that we take the maximum over i.i.d. random variables. \\
	We can conclude by basic calculations:
	\begin{align*}
	\Ex[]{\ALG} & \geq \Ex[]{\textnormal{SW}_{\textnormal{quantile}}} = \sum_{i=1}^{n} \sum_{j=1}^{n} \Ex[]{v_{i, j} X_{i, j}} \geq \frac{1}{n} \sum_{i=1}^{n} \sum_{j=1}^{n} \frac{H_{n-i+1}}{H_n} \Ex[]{\max_{i' \in [n]} v_{i', j}}
	\\ & = \frac{\sum_{i=1}^{n} H_{n-i+1}}{n H_n} \sum_{j=1}^{n} \Ex[]{\max_{i' \in [n]} v_{i', j}}  = \left( 1 - O \left( \frac{1}{\log n} \right) \right) \sum_{j=1}^{n} \Ex[]{\max_{i' \in [n]} v_{i', j}} \\ & \geq \left( 1 - O \left( \frac{1}{\log n} \right) \right)\Ex[]{\OPT}
	\end{align*}
	
\end{proof}
